# Supplementary material for: Automatic and Efficient Customization of Neural Networks for ML Applications
Source: arXiv:2310.04685 source file (2023-10-07)
Supplement: Supplementary file 3 [file revision-appendix.tex]

\onecolumn % to fit tabularx 

\section*{Appendix. }
\label{sec:revision}

\section*{Labels included in each subcategory} 

\subsection{}
